# Supplementary material for: Prometheus: An Open-Source Neutrino Telescope Simulation
Source: arXiv:2304.14526 source file (2023-04-27)
Supplement: Supplementary file 1 [file fennel_checks.tex]

\section{\texttt{Fennel} Verification}
\label{app:fennel_checks}
