# Supplementary material for: Prometheus: An Open-Source Neutrino Telescope Simulation
Source: arXiv:2304.14526 source file (2023-04-27)
Supplement: Supplementary file 2 [file ppc_tables.tex]

\section{\texttt{PPC} Tables}
\label{app:ppc_tables}
